# Supplementary material for: Embodied Referring Expression Comprehension in Human-Robot Interaction
Source: arXiv:2512.06558 source file (2025-12-06)
Supplement: Supplementary file 1 [file dataset_analyses.tex]

\section{{\dsxl} and {\dsl} Dataset Analyses}
\color{blue}
In total there are 11,617,626 scenes in the CAESAR-XL dataset and 841,620 scenes in the CAESAR-L dataset. For each scene, we sample three verbal templates from 13 templates to generate verbal utterances. In total, each scene in the CAESAR-XL dataset (as this dataset only contains RGB images and no video) contains 15 images, with 3 images of each 4 nonverbal interactions settings (human using gaze and gestures, human using only gaze, human using only gestures, human using wrong gaze and gestures) as well as 3 images with no human settings. The number of images in the CAESAR-L dataset varies due to variable length videos, but the number of still canonical frames is 30 due to the inclusion of a skeletal pose modality. The number of generated frames for the CAESAR-L dataset (which was recorded at 15 FPS), ranges from 65 to 102.
\color{black}

As the task addressed in this paper was the \textit{embodied spatial relation grounding} task, we needed to generate contrastive situations $50\%$ of the time. Fig.~\ref{fig:situation_stats} shows this, where contrastive situations represent about $50\%$ of all samples (note that the model was trained on a $50/50$ contrastive to non-contrastive sample ratio). In total, there are eight different situations contained within this task, which were discussed in the paper in Sections 3.3 and 3.6.

\begin{figure}[!t]
    \centering
    \begin{tabular}{ccc}
     \includegraphics[width=0.48\columnwidth]{latex/images/stat_images_XL/situation_frequency.png} &
     \includegraphics[width=0.48\columnwidth]{latex/images/stat_images_L/situation_frequency.png}\\
     (a) {\dsxl} & (b) {\dsl} \\
    \end{tabular}
    \caption{Distribution of different situations in the {\dsxl} and {\dsl} datasets.}
    \label{fig:situation_stats}
\end{figure}

\begin{figure}[h]
    \centering
    \begin{tabular}{cc}
     \includegraphics[width=0.47\columnwidth]{latex/images/stat_images_XL/instruction_lengths_frequency.png} & 
     \includegraphics[width=0.47\columnwidth]{latex/images/stat_images_L/instruction_lengths_frequency.png}\\
     \makecell{(a) {\dsxl} dataset.} & \makecell{(b) {\dsl} dataset.}
    \end{tabular}
    \caption{Frequency distribution of verbal utterances lengths in the {\dsxl} and {\dsxl} datasets.}
    \label{fig:verbal_expression_stats}
\end{figure}

\begin{figure}[h]
    \centering
    \begin{tabular}{cc}
     \includegraphics[width=0.45\columnwidth]{latex/images/stat_images_XL/names_frequency.png} & 
     \includegraphics[width=0.45\columnwidth]{latex/images/stat_images_L/names_frequency.png}\\
     \makecell{(a) {\dsxl} dataset.} & \makecell{(b) {\dsl} dataset.}
    \end{tabular}
    \caption{Most referred object categories in the {\dsxl} and {\dsxl} datasets.}
    \label{fig:object_category_stats}
\end{figure}

\begin{figure}[!h]
    \centering
    \begin{tabular}{cc}
        \includegraphics[clip, trim=0cm 0cm 0cm 0cm, width=0.5\textwidth]{latex/images/stat_images_XL/wordcloud.pdf} &          \includegraphics[clip, trim=1cm 15cm 1cm 1cm, width=0.5\textwidth]{latex/images/stat_images_L/wordcloud.pdf} \\
        (a) {\dsxl} dataset & (b) {\dsl} dataset
    \end{tabular}
    
    \caption{A wordcloud for all verbal expressions in the {\dsxl} and {\dsl} datasets, where the size of words represents their relative frequencies. The most frequent words describe sizes of objects, colors, and spatial relations/locations.} % Following these types of words in popularity were object names, such as pillow.
    \label{fig:wordcloud}
\end{figure}

% \begin{figure}
%     \centering
%     \begin{tabular}{c}
%      \includegraphics[width=0.7\columnwidth]{latex/images/stat_images_L/situation_frequency.png}\\
%     \end{tabular}
%     \caption{Distribution of different situations in the {\dsxl} dataset.}
%     \label{fig:situation_stats}
% \end{figure}

% reference: https://papers.nips.cc/paper/2020/file/76dc611d6ebaafc66cc0879c71b5db5c-Supplemental.pdf

% \subsection{Dataset Analyses: {\dsxl}}
% add scenarios stat analysis here
% add wrap figure for scenarios stat

\begin{figure}[!h]
    \begin{center}
    \small
    
    \begin{tabular}{c}
         \includegraphics[width=0.95\columnwidth]{latex/images/stat_images_XL/view_verbal_classification_location_lr.png}\\
        (a) Visualizing object locations for the verbal utterances containing "Left" and "Right" spatial location.\\
        \includegraphics[width=0.95\columnwidth]{latex/images/stat_images_XL/view_verbal_classification_location_fb.png}\\
        (b) Visualizing object locations for the verbal utterances containing "Front" and "Back" spatial location.\\
        \includegraphics[width=0.95\columnwidth]{latex/images/stat_images_XL/view_verbal_classification_corners.png}\\
        (c) Visualizing object locations for the verbal utterances containing four corner spatial locations.\\
        \includegraphics[width=0.95\columnwidth]{latex/images/stat_images_XL/view_verbal_classification_center.png}\\
        (d) Visualizing object Locations containing "center" term vs. all other spatial location terms.
    \end{tabular}
    \caption{Analysis of object spatial locations throughout different terms in verbal utterances in the {\dsxl} dataset. These visualizations show that the contrastive spatial locations in verbal utterances, such as \textit{left} and \textit{right}, are not separable based on the object locations in visual modalities. This property of our dataset ensures the model does not benefit from exploiting 2D visual cues and verbal modalities to ground embodied spatial relations, thus ensuring the model learns the perspective-taking necessary for real world embodied situations. Therefore, using our datasets, we can train a model that can effectively learn to attend to the salient portion of nonverbal signals to ground embodied spatial relations.}
    \label{fig:spatial_location}
    \end{center}
\end{figure}

\begin{figure}[!h]
\small
    \begin{center}
    \begin{tabular}{c}
        \includegraphics[width=0.95\columnwidth]{latex/images/stat_images_XL/view_verbal_classification_relation_lr.png}\\
        (a) Visualizing object locations for the verbal utterances containing "Left of" and "Right of" spatial relations.\\
        \includegraphics[width=0.95\columnwidth]{latex/images/stat_images_XL/view_verbal_classification_relation_fb.png}\\
        (b) Visualizing object locations for the verbal utterances containing "Front of" and "Behind" spatial relations.\\
        \includegraphics[width=0.95\columnwidth]{latex/images/stat_images_XL/view_verbal_classification_next.png}\\
        (c) Visualizing object locations for the verbal utterances containing "Next to" spatial relations.\\
    \end{tabular}
    
    \caption{Analyses of spatial relations given through verbal utterances in the {\dsxl} dataset. These visualizations show that contrastive spatial relations, such as \textit{left of} and \textit{right of}, are not separable based on object locations in the visual modalities.}
    \label{fig:spatial_relation}
    \end{center}
\end{figure}

\begin{figure}[!h]
    \begin{center}
    \small
    
    \begin{tabular}{c}
         \includegraphics[width=0.95\columnwidth]{latex/images/stat_images_L/view_verbal_classification_location_lr.png}\\
        (a) Visualizing object locations for the verbal utterances containing "Left" and "Right" spatial location.\\
        \includegraphics[width=0.95\columnwidth]{latex/images/stat_images_L/view_verbal_classification_location_fb.png}\\
        (b) Visualizing object locations for the verbal utterances containing "Front" and "Back" spatial location.\\
        \includegraphics[width=0.95\columnwidth]{latex/images/stat_images_L/view_verbal_classification_corners.png}\\
        (c) Visualizing object locations for the verbal utterances containing four corner spatial locations.\\
        \includegraphics[width=0.95\columnwidth]{latex/images/stat_images_L/view_verbal_classification_center.png}\\
        (d) Visualizing object Locations containing "center" term vs. all other locations.
    \end{tabular}
    \caption{Analyses of spatial locations through verbal utterances in the {\dsl} dataset.}
    \label{fig:spatial_location_dsl}
    \end{center}
\end{figure}

\begin{figure}[!h]
\small
    \begin{center}
    \begin{tabular}{c}
        \includegraphics[width=0.95\columnwidth]{latex/images/stat_images_L/view_verbal_classification_relation_lr.png}\\
        (a) Visualizing object locations for the verbal utterances containing "Left of" and "Right of" spatial relations.\\
        \includegraphics[width=0.95\columnwidth]{latex/images/stat_images_L/view_verbal_classification_relation_fb.png}\\
        (b) Visualizing object locations for the verbal utterances containing "Front of" and "Behind" spatial relations.\\
        \includegraphics[width=0.95\columnwidth]{latex/images/stat_images_L/view_verbal_classification_next.png}\\
        (c) Visualizing object locations for the verbal utterances containing "Next to" spatial relations.\\
    \end{tabular}
    
    \caption{Analyses of spatial relations given through verbal utterances in the {\dsl} dataset.}
    \label{fig:spatial_relation_dsl}
    \end{center}
\end{figure}

% \begin{wrapfigure}{r}{0.6\columnwidth}
%     \centering
%     \begin{tabular}{c}
%      \includegraphics[width=0.5\columnwidth]{latex/images/stat_images_XL/instruction_lengths_frequency.png}\\
%      \makecell{(a) Frequency of verbal description lengths.} \\
%      \includegraphics[width=0.5\columnwidth]{latex/images/stat_images_XL/names_frequency.png} \\
%      \makecell{(b) Frequency of referred objects.} \\
%     \end{tabular}
%     \caption{Analyses of verbal description lengths and referred object categories in the {\dsxl} dataset.}
%     \label{fig:verbal_expression_stats}
% \end{wrapfigure}

% \begin{figure}
% \scriptsize
%     \centering
%     \begin{tabular}{cc}
%      \includegraphics[width=0.5\columnwidth]{latex/images/stat_images_XL/instruction_lengths_frequency.png} & 
%      \includegraphics[width=0.5\columnwidth]{latex/images/stat_images_L/instruction_lengths_frequency.png}\\
%      \makecell{(a) Distribution of verbal utterances lengths in {\dsxl} dataset.} & \makecell{(b) Frequency of verbal description lengths ({\dsl}).} \\
%      \includegraphics[width=0.5\columnwidth]{latex/images/stat_images_XL/names_frequency.png} \\
%      \makecell{(b) Frequency of referred objects.} \\
%     \end{tabular}
%     \caption{Analyses of verbal description lengths and referred object categories in the {\dsxl} dataset.}
%     \label{fig:verbal_expression_stats}
% \end{figure}

\subsection{Object Category and Verbal Expression}

We visualize the lengths of verbal utterances and the most frequent object categories used in our generated datasets {\dsxl} and {\dsl} (Fig.~\ref{fig:object_category_stats} \& \ref{fig:verbal_expression_stats}). In Fig.~\ref{fig:object_category_stats}, all the object categories are used a similar number of times except the Knife, Cactus, and Pillow categories in the {\dsxl} dataset. These three object categories had multiple instances with different attributes (size and color) in the object library used to generate the {\dsxl} dataset (Fig.~\ref{fig:object_lib_xl}). Similarly, all object categories are used close to the same number of times in the {\dsl} dataset. As an additional verbal expression visualization, Fig.~\ref{fig:wordcloud} shows the most common words of all verbal utterances found in the {\dsxl} dataset through a wordcloud, where the largest words are the words appearing most frequently. Moreover, the worldcloud visualization indicates that the most frequent words describe sizes of objects, spatial relations, spatial
locations, and colors. % Other verbal expression metrics regarding instruction lengths and referred object frequencies can be found in Fig.~\ref{fig:verbal_expression_stats}.

\subsection{Spatial Location and Relation Visualizations}
One of the goals of {\pa} was to reduce the spatial bias from previous datasets with respect to spatial location/relation terms, as addressed in Section 4 in the paper. Particularly, we wanted to ensure models were learning the perspective-taking and nonverbal signals necessary to perform in real-world embodied situations. Thus, object locations plotted with respect to spatial location/relational terms in verbal utterances that can be used ambiguously from multiple perspectives should be non-separable, to ensure models do not bias verbal utterances or 2D visual cues during training (Fig.~\ref{fig:spatial_location}, \ref{fig:spatial_relation},\ref{fig:spatial_location_dsl}, \ref{fig:spatial_relation_dsl}). Aligning with this, Figs.~\ref{fig:spatial_location} \& \ref{fig:spatial_location_dsl} show visualizations for different terms when specifying object spatial locations, where the only locational term with separable points being the spatial location "center". This makes sense as the center is the only locational term used in {\pa} that is objective from both the exo and ego perspectives. Similarly, Figs.~\ref{fig:spatial_relation} \&  \ref{fig:spatial_relation_dsl} show visualizations for different terms when specifying object spatial relations, where no terms provide a separable pairs of points. Please note that the term "Next to" is not compared to any other terms as it is a standalone term used in all locations with no complements, and thus does not lead to model bias or point separability. 

% \begin{figure}[!t]
%     \centering
%     \includegraphics[clip, trim=1cm 10cm 1cm 1cm, width=0.5\textwidth]{latex/images/stat_images_L/wordcloud.pdf}
    
%     \caption{A wordcloud for all verbal expressions in {\dsxl} and {\dsl} datasets, where the size of words represents their relative frequencies. The most popular words described object relations/locations, size, and color. Following these types of words in popularity were object names, such as pillow.}
%     \label{fig:wordcloud}
% \end{figure}

% \subsection{Dataset Analyses: {\dsl}}

% \subsubsection{Spatial Location and Relation Visualizations}

% \subsection{Verbal Expression}
