# Supplementary material for: Embodied Referring Expression Comprehension in Human-Robot Interaction
Source: arXiv:2512.06558 source file (2025-12-06)
Supplement: Supplementary file 2 [file datasets_source_code_access.tex]

\section{Access to Datasets, Source Codes, Benchmark Model Checkpoints, and Docker}
The datasets we generated, source code for our simulator, benchmark learning models, trained model checkpoints, and simulator configuration guide can be accessed through the following links. These resources are only shared with reviewers. We will publicly release these resources with the camera-ready version of our paper.

\begin{itemize}
    \item \textbf{Project website: }\\ \url{https://caesar-simulator.github.io}
    \item \textbf{{\dsxl} dataset ($319$ GB):}\\ \url{https://drive.google.com/file/d/13KAUBxW3jdu3RuUQMuJCamdNMa59gyXv}
    \item \textbf{{\dsl} dataset ($181$ GB):}\\ \url{https://drive.google.com/file/d/1Q_kybqktCjthuIuWU01-l15muby69izq}
    \item \textbf{CAESAR-S dataset ($5.31$ GB):}\\ \url{https://drive.google.com/file/d/1eppJrUfxLNPQsY8s1ItsSlrYPRgJ6T0l}
    \item \textbf{Source code of data processing, and benchmark learning models:}\\ \url{https://drive.google.com/drive/folders/1HRZrYgxDNi1wv9s0hNFBPJt51FACHgss}
    \item \textbf{Trained model checkpoints ($3.54$ GB):}\\ \url{https://drive.google.com/drive/folders/1kqCbNwPlO5gq4n0Q8Jo3UFGodSfwzwn_}
    \item \textbf{Docker for computing environment ($6.84$ GB):}\\ \url{https://hub.docker.com/r/mmiakashs/pytorch_1-11_pl_1-6-1}
    \item \textbf{Source code of the {\pa} simulator ($11.8$ GB):}\\ \url{https://drive.google.com/file/d/1y8nBkE3G9Ppq7vwWRMYBmTdWbaE6IyG8}
    \item \textbf{The {\pa} simulator installation guide:}\\ \url{https://drive.google.com/file/d/1_NixyzRAuedGy6U9Ngy14PkzGGgFqOay}
    \item \textbf{The {\pa} simulator configuration and data generation tool guide:} \\ \url{https://youtu.be/KnKcpG7c2fk}
\end{itemize}

\color{blue}
\section{Source code and Datasets Accessibility}
We use GitHub to host and publicly release all the source code for simulator, dataset parsing, and benchmark model experimentation. We will release the future versions of our simulator through GitHub. We highly encourage other researchers to create a pull request to update the simulator, issue bugs, or resolve any known bugs. Additionally, researchers can request additional features by contacting us. 

We host our datasets in two places: Google Drive and University of Virginia’s secure storage system (Rivanna: https://www.rc.virginia.edu/userinfo/storage/). As the Rivanna storage system periodically backs the storage up, this storage is safer and ideal for long-term storage. We will share the datasets with other researchers via the Google drive links or provide read-access to the Rivanna storage system using the Globus File sharing system (https://www.globus.org/data-sharing). Additionally, As our generated datasets are large in size, if researchers prefer, we can share the dataset via storage drives. However, the researchers need to bear a fixed charge to cover the cost of the storage drive and standard shipping. 
The authors of the paper maintain both of the generated datasets. Contact information: Md Mofijul Islam (Email: mi8uu@virginia.edu) and Prof. Tariq Iqbal (tiqbal@virginia.edu). 

\color{black}
