# Supplementary material for: Embodied Referring Expression Comprehension in Human-Robot Interaction
Source: arXiv:2512.06558 source file (2025-12-06)
Supplement: Supplementary file 3 [file datasheets.tex]

\section{Access to Datasets, Source Codes, Benchmark Model Checkpoints, and Docker}
The datasets we generated, source code for our simulator, benchmark learning models, trained model checkpoints, and simulator configuration guide can be accessed through the following links. These resources are only shared with reviewers. We will publicly release these resources with the camera-ready version of our paper.

\begin{itemize}
    \item \textbf{Project website: }\\ \url{https://caesar-simulator.github.io}
    \item \textbf{{\dsxl} dataset ($319$ GB):}\\ \url{https://drive.google.com/file/d/13KAUBxW3jdu3RuUQMuJCamdNMa59gyXv}
    \item \textbf{{\dsl} dataset ($181$ GB):}\\ \url{https://drive.google.com/file/d/1Q_kybqktCjthuIuWU01-l15muby69izq}
    \item \textbf{CAESAR-S dataset ($5.31$ GB):}\\ \url{https://drive.google.com/file/d/1eppJrUfxLNPQsY8s1ItsSlrYPRgJ6T0l}
    \item \textbf{Source code of data processing, and benchmark learning models:}\\ \url{https://drive.google.com/drive/folders/1HRZrYgxDNi1wv9s0hNFBPJt51FACHgss}
    \item \textbf{Trained model checkpoints:}\\ \url{https://drive.google.com/drive/folders/1kqCbNwPlO5gq4n0Q8Jo3UFGodSfwzwn_}
    \item \textbf{Docker for computing environment:}\\ \url{https://hub.docker.com/r/mmiakashs/pytorch_1-11_pl_1-6-1}
    \item \textbf{Source code of the {\pa} simulator (11.8 GB):}\\ \url{https://drive.google.com/file/d/1y8nBkE3G9Ppq7vwWRMYBmTdWbaE6IyG8}
    \item \textbf{The {\pa} simulator installation guide:}\\ \url{https://drive.google.com/file/d/1_NixyzRAuedGy6U9Ngy14PkzGGgFqOay}
    \item \textbf{The {\pa} simulator configuration and data generation tool guide:} \\ \url{https://youtu.be/KnKcpG7c2fk}
\end{itemize}

\section{Author Statement}
Our datasets can be accessed using the CC BY-NC-SA license (\url{https://creativecommons.org/licenses/by-nc-sa/4.0/}). Moreover, our simulator source code will be released under the BSD 3-Clause license (\url{https://opensource.org/licenses/BSD-3-Clause}).

\section{Motivation}

\textbf{For what purpose was the dataset created? Was there a specific task in mind? Was there a specific gap that needed to be filled? Please provide a description.}

% This dataset was created for the purpose of training multimodal machine learning models on embodied referring expression in the hopes of these models being generalizable/transferrable to the real world in the future. 

We developed an embodied simulator, {\pa}, to generate large-scale datasets of embodied referring expressions. Existing data generation tools can not generate embodied reference expression with verbal utterances and nonverbal gestures. Moreover, existing datasets of embodied referring expressions only capture nonverbal interactions from an exocentric perspective. To the best of our knowledge, {\pa} is the first simulator to generate multimodal referring expressions with verbal utterances and nonverbal gestures in a virtual environment. Our generated datasets can be used to understand embodied multimodal referring expressions from multiple perspectives.

The {\pa} simulator has three novel aspects that differentiate it from other synthetic data generation systems. First, {\pa} simulates scenarios in which verbal utterances and nonverbal cues (pointing gesture and gaze) refer to objects in an embodied setting. We have collected real human pointing gesture data using an OptiTrack motion capture system and emulated the same behaviors in the {\pa} simulator by incorporating a new stochastic deictic gesture generation approach. Second, the {\pa} simlator renders multiple views from three different perspectives: the ego-, exo-, and top-view, that can aid in training models to learn different perspectives for comprehending multimodal referring expressions. Third, we have designed a module in the {\pa} simulator to generate contrastive samples, where the virtual human is pointing to an object while verbally describing a different object. 

\textbf{Who created the dataset (e.g., which team, research group) and on behalf of which entity (e.g., company, institution, organization)?}

Every author in this paper contributed in developing the datasets and benchmarking models. The authors are with the Collaborative Robotics Lab at the University of Virginia.

% \textcolor{green}{\textbf{Who funded the creation of the dataset? If there is an associated grant, please provide the name of the grantor and the grant name and number.}}

\section{Composition}

\textbf{What do the instances that comprise the dataset represent (e.g., documents, photos, people,
countries)? Are there multiple types of instances (e.g., movies, users, and ratings; people and
 interactions between them; nodes and edges)? How many instances are there in total (of each
 type, if appropriate)?}
 
 Each instance represents a different scene that a simulator generated, where a human nonverbally and verbally refers to an object in a simulated environment. Each instance of the{\dsl} dataset contains videos, images, and skeletal modalities to capture nonverbal interactions from three views (ego, exo, and top). Each instance also contains a verbal expression to describe the referred object. Additionally, each instance of the {\dsxl} dataset contains images of nonverbal interactions from the three views (ego, exo, and top) as well as a verbal expression. There are a total of $1,367,305$ instances in the {\dsxl} dataset and $124,412$ instances in the {\dsl} dataset. The {\dsl} dataset consists of $124,412$ data samples created from $11,617,626$ images at a resolution of $480\times320$ pixels. The {\dsxl} dataset consists of $1,367,305$ data samples, which were created from $841,620$ images by varying verbal expressions in five different settings. These images were rendered with a resolution of $720\times480$ pixels using an object pool of size $80$. The details of these datasets have been presented in the paper and in the supplementary document.
 
\textbf{Does the dataset contain all possible instances or is it a sample (not necessarily random) of instances from a larger set?}
 
 These datasets contain all possible instances. 
 %We have generated diverse data by varying the verbal and nonverbal modalities. We have generated a verbal description of an object from five verbal templates described in the paper and in the supplementary document. We have generated data for three scenarios - a person gazing at an object, a person pointing to an object, and a person gazing and pointing at an object. Additionally, we have generated contrastive data of these scenarios where verbal and nonverbal expressions refer to different objects.
 
\textbf{What data does each instance consist of? “Raw” data (e.g., unprocessed text or images) or
 features? In either case, please provide a description.}
 
Each data instance of the {\dsxl} dataset contains images from three views (ego, exo, and top) to capture nonverbal interaction and verbal descriptions of the referred object. Each data instance of the {\dsl} dataset contains videos, images, and skeletal from three views (ego, exo, and top) to capture nonverbal interactions, as well as a verbal description of the referred object. 
 
\textbf{Is there a label or target associated with each instance?}

Yes. We have provided the label of each data sample to indicate whether the generated multimodal referring expressions (verbal and nonverbal) refer to the same object. This is contained in the data.json file for every data sample.

\textbf{Is any information missing from individual instances? If so, please provide a description,
explaining why this information is missing (e.g., because it was unavailable). This does not
include intentionally removed information, but might include, e.g., redacted text.}

No information is missing from individual instances.

\textbf{Are relationships between individual instances made explicit (e.g., users’ movie ratings, social
 network links)? If so, please describe how these relationships are made explicit.}
 
Yes. We have provided detailed annotations of each generated data sample, as described in the supplementary document.

\textbf{Are there recommended data splits (e.g., training, development/validation, testing)? If so,
 please provide a description of these splits, explaining the rationale behind them.}
 
 Yes, we have provided three data splits (train, test, validation) in three separate csv files (train.csv, test.csv, valid.csv) for each dataset ({\dsl} and {\dsxl}). The rationale behind splitting the data as such was to ensure model training repeatability.

\textbf{Are there any errors, sources of noise, or redundancies in the dataset? If so, please provide a
 description.}
 
 We have comprehensively tested the simulator for error or noise, including having humans verify hundreds of data samples. There are currently no known bugs or sources of noise in the simulator and consequentially no known errors in the datasets.
 In the future, if we find additional errors or noise, we will rectify those errors and release an updated version on our project website.
 %carefully developed the simulator and generated datasets without any error and noise. 
 
\textbf{Is the dataset self-contained, or does it link to or otherwise rely on external resources (e.g.,
 websites, tweets, other datasets)? If it links to or relies on external resources,}
 
 Our generated datasets, ({\dsl} and {\dsxl}), are self-contained. We provided the generated data, including images, video, skeletal, and verbal modalities. %If anyone desires to generate new datasets, they may do so through downloading the source code of our simulator and generating data, as described further in our supplementary.  
 
\textbf{Does the dataset contain data that might be considered confidential (e.g., data that is protected
by legal privilege or by doctor patient confidentiality, data that includes the content of individuals’ non-public communications)?}

No, the datasets contain generated synthetic data and thus do not contain data that might be considered confidential.

\textbf{Does the dataset contain data that, if viewed directly, might be offensive, insulting, threatening,
 or might otherwise cause anxiety?}

No.

\textbf{Does the dataset relate to people? If not, you may skip the remaining questions in this section.}

No. Our datasets contain generated human avatars from a library of eight avatars presented in the supplementary document and source code of the simulator.

\textbf{Does the dataset identify any subpopulations (e.g., by age, gender)? If so, please describe how
 these subpopulations are identified and provide a description of their respective distributions
 within the dataset.}
 
No. As we synthetically generated the datasets, no subpopulations are identified.

\textbf{Is it possible to identify individuals (i.e., one or more natural persons), either directly or indirectly (i.e., in combination with other data) from the dataset?}

No, no individuals can be identified as we used humanoid avatars.

\textbf{Does the dataset contain data that might be considered sensitive in any way (e.g., data that reveals racial or ethnic origins, sexual orientations, religious beliefs, political opinions or union memberships, or locations; financial or health data; biometric or genetic data; forms of government identification, such as social security numbers; criminal history)?}

No. Datasets contains generated data with virtual human avatars and synthetic objects. We include diverse avatars to remove the racial/gender bias in the dataset.

\section{Preprocessing, cleaning and labeling}

\textbf{Was any preprocessing/cleaning/labeling of the data done (e.g., discretization or bucketing,
 tokenization, part-of-speech tagging, SIFT feature extraction, removal of instances, processing
 of missing values)? If so, please provide a description. If not, you may skip the remainder of
 the questions in this section.}
 
Some cleaning of the dataset was done by filtering out samples without the required labels (data.json). These samples were very few and are not present in the training/testing/validation csv files. We have provided the source code to filter these data samples: \url{https://drive.google.com/drive/folders/1HRZrYgxDNi1wv9s0hNFBPJt51FACHgss}.
 
\textbf{Was the “raw” data saved in addition to the preprocessed/cleaned/labeled data (e.g., to support
 unanticipated future uses)? If so, please provide a link or other access point to the “raw” data.}

Yes. We have provided all the raw data of images, video, skeletal, and verbal modalities.

\textbf{Is the software used to preprocess/clean/label the instances available? If so, please provide a
 link or other access point.}
 
 Yes. We used various Python packages, such as pandas, numpy, and matplotlib, to process raw data \footnote{Pandas: https://pandas.pydata.org/, Numpy: https://numpy.org/, Matplotlib: https://matplotlib.org/}.

\section{Use Cases}

\textbf{Has the dataset been used for any tasks already? If so, please provide a description.}

We have designed an \textit{embodied spatial relation grounding task}, which involves identifying whether a person is verbally and nonverbally (pointing gesture and gaze) referring to the same objects in the visual scene. This task can help develop learning frameworks to understand multimodal referring expressions in embodied settings. We evaluated several models on our {\dsxl} dataset by varying modalities, perspectives, and fusion methods. 

\textbf{Is there a repository that links to any or all papers or systems that use the dataset? If so, please  provide a link or other access point. What (other) tasks could the dataset be used for?}
 
At the top of this pdf are links for all the models/systems that use this dataset. In this work, we have developed several benchmark models and evaluated on our dataset for embodied spatial relation grounding task. This dataset could be used for other tasks related to multimodal embodied referral expression, including bounding box detection, skeletal pose identification, and many other tasks.

We believe that datasets generated from our simulator can be used to train and evaluate models for various tasks in embodied settings, such as embodied question answering, object grounding, and conversational human-AI interactions. Moreover, these datasets can be used to pre-train models for embodied instruction comprehension, which can be transferred to robots for comprehending instructions to seamless human-robot interactions in real-world settings.
 
\textbf{Is there anything about the composition of the dataset or the way it was collected and preprocessed/cleaned/labeled that might impact future uses?}

We have described the composition of the dataset in the paper and the supplementary document.

\textbf{Are there tasks for which the dataset should not be used? If so, please provide a description.}

No, not applicable.

\section{Distribution}

\textbf{Will the dataset be distributed to third parties outside of the entity (e.g., company, institution,
 organization) on behalf of which the dataset was created? If so, please provide a description.}

Yes, researchers can use our dataset free of cost after signing a data use agreement (DUA). Moreover, researchers can also use our simulator to generate datasets according to their needs.

\textbf{How will the dataset will be distributed (e.g., tarball on website, API, GitHub)? Does the dataset have a digital object identifier (DOI)?}
 
We will share the dataset using Google Drive after receiving a data use agreement (DUA). We have a plan to create digital object identifier (DOI) after releasing datasets and simulator.

\textbf{When will the dataset be distributed?}

Our generated datasets can be accessed through the following links. These resources are only shared with the NeurIPS-2022 reviewers. We will publicly release these resources in October 2022.

\begin{itemize}
    \item \textbf{{\dsxl} Dataset:} \\
    \url{https://drive.google.com/file/d/13KAUBxW3jdu3RuUQMuJCamdNMa59gyXv}
    \item \textbf{{\dsl} Dataset:} \\
    \url{https://drive.google.com/file/d/1Q_kybqktCjthuIuWU01-l15muby69izq}
\end{itemize}

\textbf{Will the dataset be distributed under a copyright or other intellectual property (IP) license,
 and/or under applicable terms of use (ToU)? If so, please describe this license and/or ToU, and
 provide a link or other access point to, or otherwise reproduce, any relevant licensing terms or
 ToU, as well as any fees associated with these restrictions.}
 
 Our datasets can be accessed using CC BY-NC-SA license (\url{https://creativecommons.org/licenses/by-nc-sa/4.0/}). Moreover, our simulator source code will be released under BSD 3-Clause license (\url{https://opensource.org/licenses/BSD-3-Clause}).
 
 \textbf{Have any third parties imposed IP-based or other restrictions on the data associated with the
 instances? If so, please describe these restrictions, and provide a link or other access point to,
 or otherwise reproduce, any relevant licensing terms, as well as any fees associated with these
 restrictions.}
 
 No, not Applicable.

 \textbf{Do any export controls or other regulatory restrictions apply to the dataset or to individual
 instances? If so, please describe these restrictions, and provide a link or other access point to,
 or otherwise reproduce, any supporting documentation.}
 
 Not Applicable
 
 \textbf{Who is supporting/hosting/maintaining the dataset? How can the owner/curator/manager of
 the dataset be contacted (e.g., email address)?}
 
The authors of the paper are maintaining both of the generated datasets. Contact person: Md Mofijul Islam (Email: mi8uu@virginia.edu) and Prof. Tariq Iqbal (tiqbal@virginia.edu).

\textbf{Is there an erratum? If so, please provide a link or other access point.}

Not Applicable.

\textbf{Will the dataset be updated (e.g., to correct labeling errors, add new instances, delete in
stances)? If so, please describe how often, by whom, and how updates will be communicated
 to users (e.g., mailing list, GitHub)?}
 
 Yes, we will update is as often as we find issues. If we find any issues and update the dataset or simulator, we will release the updated datasets and simulator through our project website.
 
 \textbf{If the dataset relates to people, are there applicable limits on the retention of the data associated with the instances (e.g., were individuals in question told that their data would be retained
 for a fixed period of time and then deleted)? If so, please describe these limits and explain how
 they will be enforced.}
 
 Not applicable. We generated synthetic dataset using human avatars.
 
 \textbf{Will older versions of the dataset continue to be supported/hosted/maintained? If so, please
 describe how. If not, please describe how its obsolescence will be communicated to users.}
 
 We stored all the datasets in the University of Virginia Research Computing System (Rivanna). We will host all the versions of our datasets using Rivanna storage. Researchers can contact either Md Mofijul Islam (mi8uu@virginia.edu) or Prof. Tariq Iqbal (tiqbal@virginia.edu) to get access to any of the versions of the datasets.
 
 \textbf{If others want to extend/augment/build on/contribute to the dataset, is there a mechanism for them to do so? If so, please provide a description. Will these contributions be validated/verified? If so, please describe how. If not, why not? Is there a process for communicating/distributing these contributions to other users? If so, please provide a description.}
 
 We will be happy to get contributions from other researchers to extend our datasets and simulator. They can contact us with the plan of extensions. We have a plan to release our simulator source code on GitHub, and we will follow issue-based development to extend our simulator further to meet other researchers' demands.
