# Supplementary material for: Embodied Referring Expression Comprehension in Human-Robot Interaction
Source: arXiv:2512.06558 source file (2025-12-06)
Supplement: Supplementary file 4 [file human_subject_study.tex]

\section{Human-Subject Study}
We conducted a study on Amazon Mechanical Turk (MTurk) to evaluate the model. $300$ data samples were collected in which participants looked at an image from the exo view and answered a survey question on their observations. All participants were located in the United States and at least 18 years of age or older. Participants were also required to have a Human Intelligence Task (HIT) approval rating approval rating of $95\%$ or greater. Moreover, to obtain a variety of participant responses, participants were limited to three tasks. Participants were compensated $\$0.02$ for the $10$ second task.

To generate the task, we uploaded a CSV file containing the links for the $300$ exo view images to MTurk. The CSV file also contained the verbal descriptions for the images and whether the verbal and non-verbal descriptions were in contrast. MTurk randomized the order in which the images were shown. We performed three trials of the study on MTurk, so each image was shown to three participants for a total of $900$ evaluations.

The participants were first instructed to review the electronic study information document for consent and the task instructions. In the task, participants were asked to determine whether the person was verbally and non-verbally (pointing, gaze, etc.) describing the same object. Prior to the task, participants were shown examples for cases in which the person \textit{was} and \textit{was not} verbally and non-verbally identifying the same object (Fig.~\ref{mturk_study_sample}). 

\begin{figure}[t]
\centering
\includegraphics[width=0.85\columnwidth]{latex/images/mturk_study_sample.png}
\caption{Instructions given to the Amazon Mechanical Turk participants.}
\label{mturk_study_sample}
\vspace{-0.2in}
\end{figure}

\begin{figure}[t]
\centering
\includegraphics[width=0.65\columnwidth]{latex/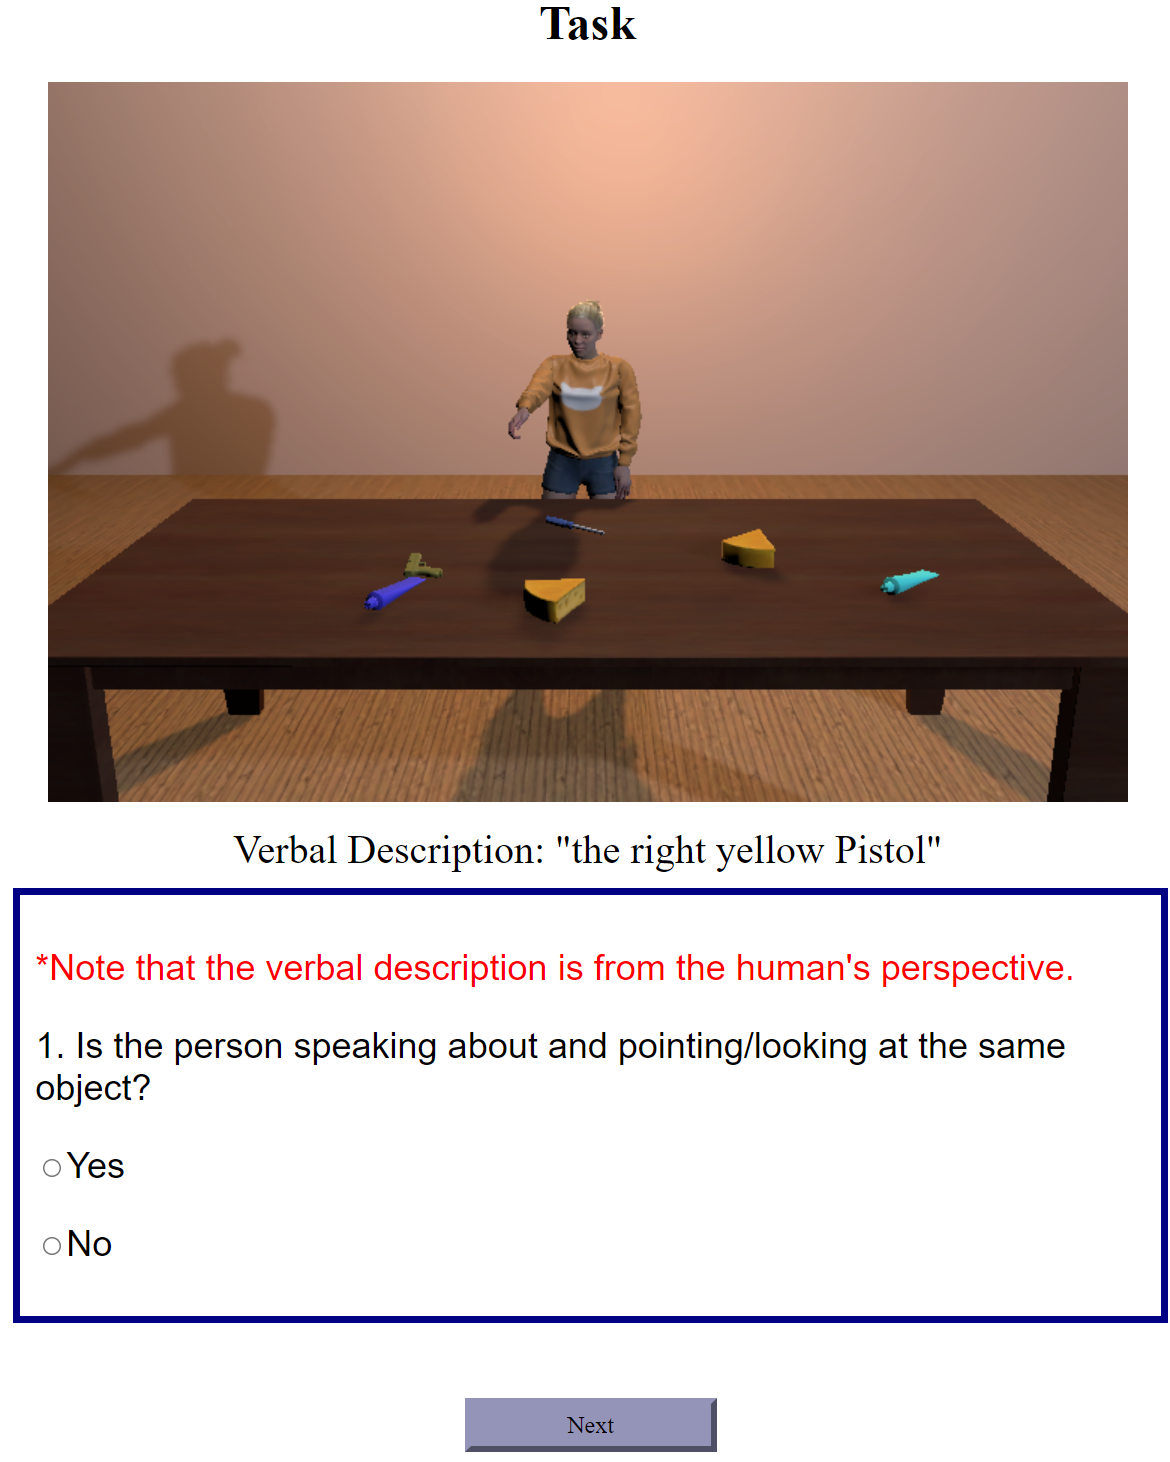}
\caption{A sample task shown to the Amazon Mechanical Turk participants.}
\label{fig:mturk_study_sample_task}
\vspace{-0.2in}
\end{figure}

During the task, participants were shown the exo view image, the verbal instruction, and a reference image containing the potential objects (Fig.~\ref{fig:mturk_study_sample_task}). After completing the task, participants were debriefed and compensated. The results of the study suggest that the participants correctly validated the relations $80.66\%$ of the time.

% \begin{figure}[t]
% \centering
% \includegraphics[width=0.85\columnwidth]{latex/images/objects_L.png}
% \caption{\textcolor{red}{Insert Caption.}}
% \label{object_list}
% \vspace{-0.2in}
% \end{figure}
