# Supplementary material for: Embodied Referring Expression Comprehension in Human-Robot Interaction
Source: arXiv:2512.06558 source file (2025-12-06)
Supplement: Supplementary file 5 [file models.tex]

\begin{figure}
    \centering
    \begin{tabular}{c}
        \includegraphics{latex/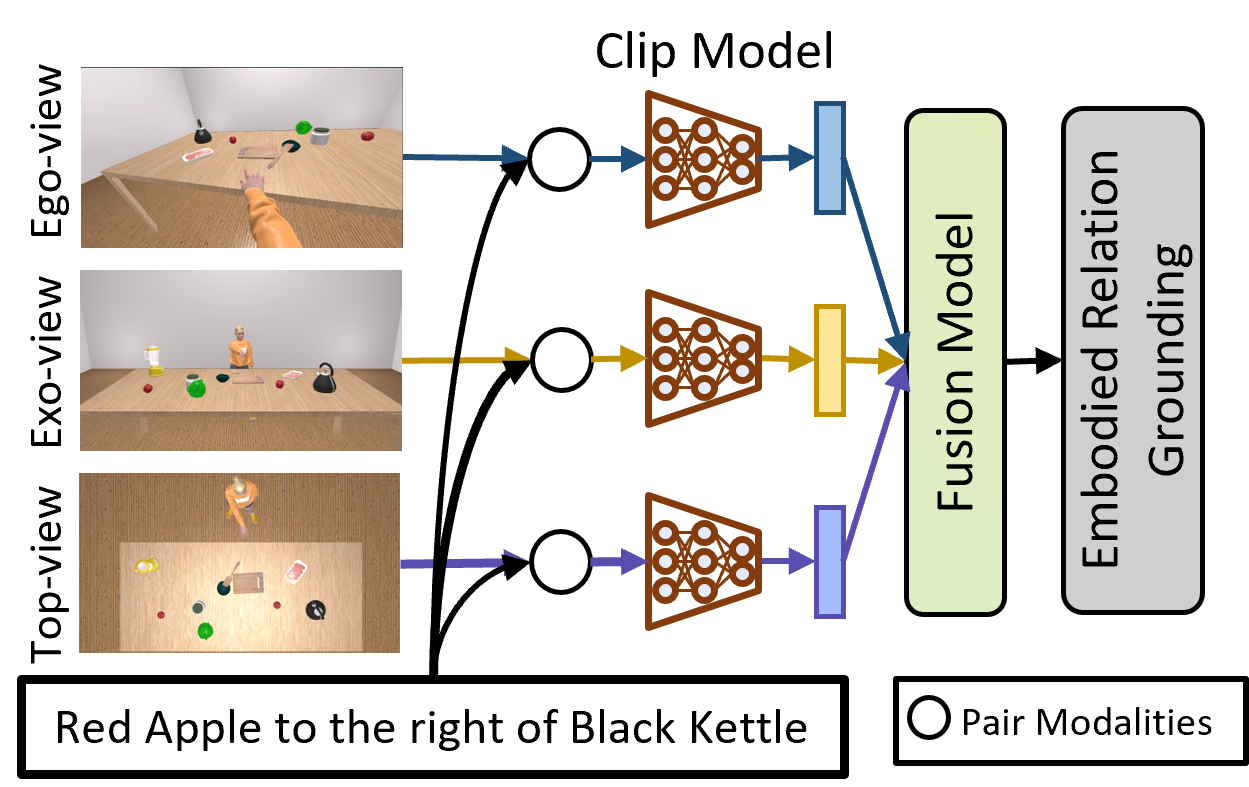} \\
        (a) Clip Model \\
        \includegraphics{latex/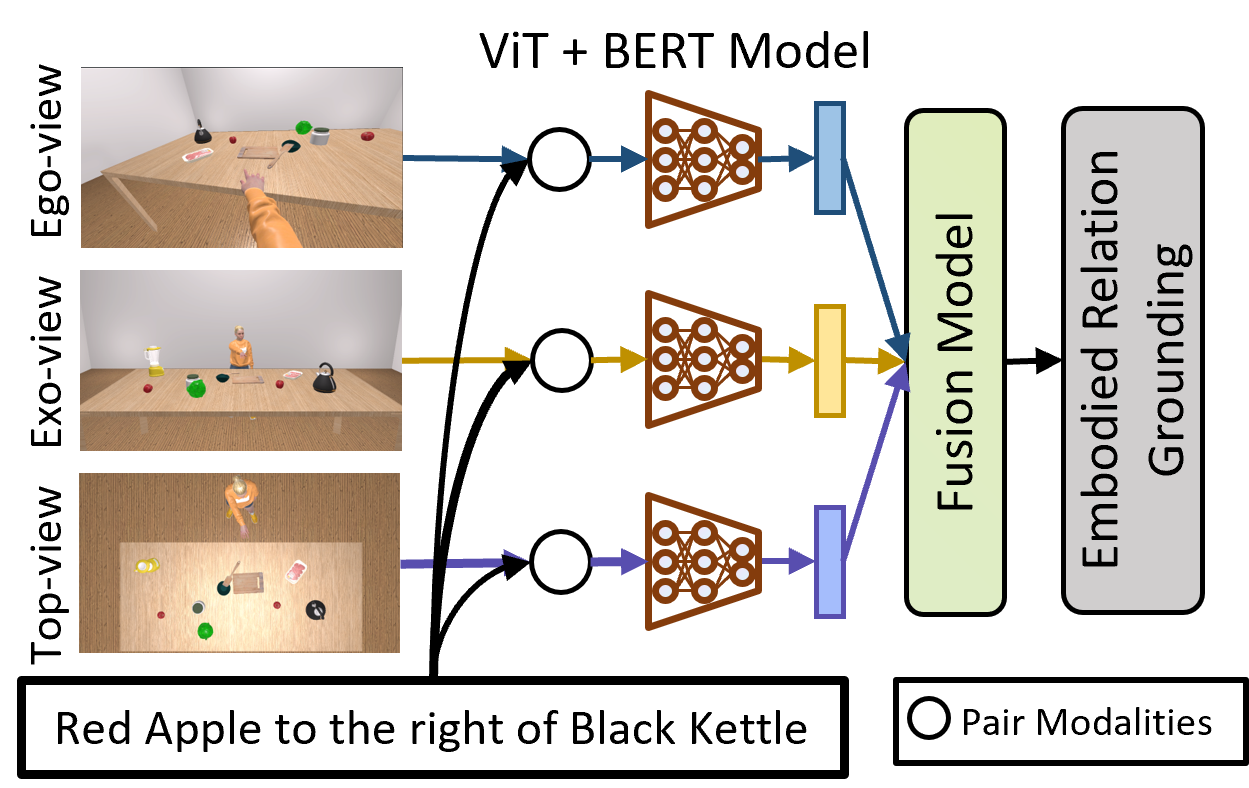} \\
        (b) Dual Encoder (ViT+BERT) \\
        \includegraphics{latex/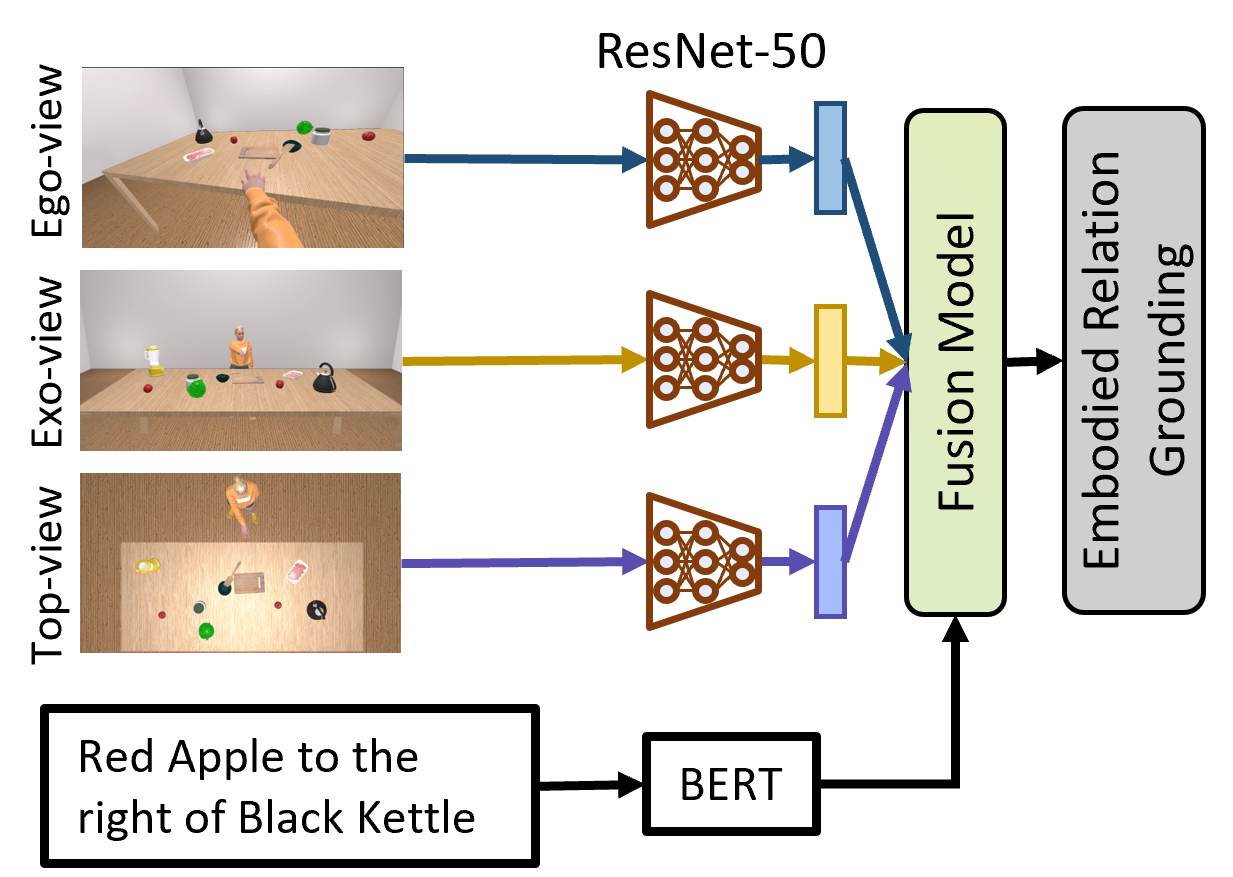} \\
        (c) Late Fusion Model (ResNet + BERT) \\
    \end{tabular}
    
    \caption{(a) Clip model takes a pair of  image, capturing nonverbal interactions, and verbal descriptions of the referred object. The clip model produces a pair of visual and verbal representations for each pair of image and verbal data. All the extracted representations are fused to produce multimodal representations for embodied relation grounding. (b) The Dual-Encoder takes a pair of image and verbal descriptions and produces a pair of verbal and visual representations, similar to the Clip models. However, Dual-Encoder model uses ViT and BERT models to encode visual and verbal modalities. (c) Late Fusion model independently encodes visual modalities using ResNet-50 model. Late Fusion model encodes verbal modalities using a pre-trained BERT model.}
    \label{fig:models}
\end{figure}

\section{Embodied Relation Grounding Models}
We have adopted visual-language models to develop three representation learning models for the embodied spatial relation grounding task: a CLIP Model \cite{clip}, a Dual-Encoder (ViT \cite{vit} + BERT \cite{bert}) model and a Late Fusion (ResNet \cite{resnet} + BERT \cite{bert}) model (Fig.~\ref{fig:models}).

\textbf{CLIP-based Model: } The CLIP model excels at aligning visual and language modalities \cite{clip}. Thus, we use the CLIP model to detect whether nonverbal cues and verbal utterances of an embodied expression refer to the same object. The CLIP model architecture processes an image-text pair and produces verbal and visual representations. For this reason, we pair the verbal expression, $T$, to each of the views of the nonverbal expression (Ego $(V_{ego})$, Exo $(V_{exo})$, and Top $(V_{top})$) and pass each modality pair to CLIP models: $E^{v}_{i}, E^{t}_{i} = CLIP(V_{i}, T) &,& i \in (ego, exo, top)$. Here, $E^{v}_{i} \in \mathbb{R}^{B \times S}$ and $E^{t}_{i} \in \mathbb{R}^{B \times S}$ are the visual and verbal embeddings from CLIP models, respectively ($B$ is the batch size and $S$ is the embedding dimension). The adopted CLIP model architecture is depicted in Fig.~\ref{fig:models}(a).

We used a Huggingface library \cite{wolf-etal-2020-transformers} to implement the CLIP model. We also used the CLIPProcessor to tokenize the input verbal data as well as process the visual data and produce the input tensors. Finally, these processed data were fed into the CLIP model to extract verbal and visual embeddings. The verbal embedding is the projected pooled output of a CLIPTextModel. Similarly, The visual embedding is the projected pooled output of a CLIPVisionModel. Both verbal and visual embeddings were a tensor of length $512$. 

\textbf{Dual-Encoder Model: } Similar to CLIP models, we pass each pair of visual and verbal modalities to Dual-Encoder models to extract verbal and nonverbal representations (Fig.~\ref{fig:models}(b)). We used ViT and BERT in a Dual-Encoder model to encode visual and verbal modalities, respectively. The ViT model (\textit{google/vit-base-patch16-224})we used was pretrained on a Huggingface library. We also used a BERT pretrained model (\textit{bert-base-uncased}) from Huggingface. This Dual-Encoder Model is pretrained to align visual-text embeddings using a CLIP like contrastive image-text training approach for zero-shot training tasks, such as image classification and image retrieval. The verbal embedding is the projected pooled output of the language model portion of the Dual-Encoder model. Similarly, The visual embedding is the projected pooled output of the vision model aspect of the Dual-Encoder model. Both verbal and visual embeddings are a tensor with length $768$. 

%Finally, in both Dual-Encoder and Late Fusion models, the encoded visual and verbal representations are fused using either of the fusion approaches described in Section~\ref{sec:clip-model} (SUM, CONCAT, Self-Attention, and Cross-Attention).

\textbf{Late Fusion Model: } In the Late Fusion model all the visual and verbal modalities are encoded independently using ResNet-50 \cite{resnet} and BERT \cite{bert} language models. First, we independently encode all the visual data modalities using a pretrained ResNet-50 model on ImageNet. Second, we encode verbal data modalities using a pretrained BERT model (\textit{bert-base-uncased}) from a Huggingface pretrained library. We projected the extracted verbal and visual modalities representations to a fixed-sized embedding of $768$.

\textbf{Multimodal Fusion:} We fused the extracted verbal and visual representations from the above-mentioned models to produced multimodal representations, which are used to detect embodied spatial relations. We used four fusion approaches: SUM, CONCAT, Self-Attention, and Cross-Attention. The first two fusion approaches summed and concatenated the verbal and visual representations. The self-attention approach is similar to the transformer-style self-attention \cite{transformer} which attends each of the verbal and visual representations and sums the attended representations. In our implementation of the self-attention model, we used $4$ heads and single layers of multi-head attention models from PyTorch. We also used a dropout of $0.1$ in this cross-attention model. We have also employed a Cross-Attention approach, which is similar to the co-attention approach from ViLBERT \cite{lu2019vilbert}. Cross-Attention is essentially a query-key-value style attention approach, where verbal embeddings are used as queries and visual embeddings are used as keys and values. In our implementation of the cross-attention model, we used $4$ heads and a single layer of multi-head attention model from PyTorch, with a dropout of $0.1$ in this cross-attention model. Finally, the fused embedding is passed through a multilayer perceptron to detect embodied spatial relations.

% , $(E^{v}=(E^{v}_{ego}, E^{v}_{exo}, E^{v}_{top}))$
% In our implementation, as the CLIP models generate multiple verbal embeddings for each verbal and visual pair, we have summed the verbal embeddings to produce query representation.

\textbf{Model Training Environment Setup:} We projected the visual and verbal embeddings from CLIP, Dual-Encoder, and Late Fusion models to $512$, $768$, and $768$ sized embeddings, respectively. We fused all the embeddings from multiple views and passed them through a multilayer perceptron to classify whether verbal and nonverbal expressions referred to the same object. We used the PyTorch-1.7 and PyTorch-Lightning-1.0.8 deep learning frameworks to implement models for training on the {\dsxl} dataset. We used the Adam optimizer with weight decay regularization, and cosine annealing warm restarts \cite{adamw} with an initial learning rate set to $3e^{-4}$ to train the evaluated approaches. To train the learning model, we set both the cycle length ($T_0$) and cycle multiplier ($T_{mult}$) to $2$. We used a batch size $8$ to train the model. We trained each evaluated model for $4$ epochs on the {\dsxl} dataset, using cross-entropy loss. We trained all the models in a distributed GPU cluster environment, where each node contains 4-8 GPUs. Please check the source code for further details of the model implementations. We have also released a docker container to replicate the execution environment (6.84 GB):\\ \url{https://hub.docker.com/r/mmiakashs/pytorch_1-11_pl_1-6-1}.
