# Supplementary material for: Embodied Referring Expression Comprehension in Human-Robot Interaction
Source: arXiv:2512.06558 source file (2025-12-06)
Supplement: Supplementary file 6 [file simulator.tex]

\begin{figure}[!h]
    \centering
    \includegraphics[clip, trim=1.5cm 12cm 1.5cm 7cm, width=0.9\textwidth]{latex/images/stat_images_XL/uml.drawio.pdf}
    \caption{{\pa} simullator class diagram. One SuperManager instantiates different SceneManagers depending on the number of parallel scenes designated by the user. Each scene manager is then responsible for interactions between classes, managing different modules of the simulator including generating objects, generating human gestures, recording multiple views, generating verbal expressions, and serializing all labeled data.}
    \label{fig:class-diagram}
\end{figure}

\section{CAESAR: An Embodied Simulator}

\subsection{{\pa} Simulator Structure}
We visualize the general code structure of the {\pa} simulator in a class diagram shown in Fig.~\ref{fig:class-diagram}. During the data generation process in the {\pa} simulator, there is one SuperManager class that controls the start and stop of data generation as well as the spawning of each scene. The SuperManager class spawns the number of scenes designated to run in parallel, inputted by the user through the parameter \textit{Parallel Scenes} in Table~\ref{tab:configuration_settings}, where each scene is represented by a SceneManager class. Each SceneManager class controls all the other modules of a given scene, starting with the spawning of objects via the ObjectManager class. After all objects are spawned in, the SceneManager class activates the BoneRenderer class and starts recording from multiple views via the RecordingManager class. To start creating different nonverbal embodied referral expressions, the GestureManager class is called with varying parameters (gaze and gesture). The GestureManager class uses the BezierTargetDriver class to generate pointing gestures, using the hybrid approach described in Section 3.2 in the paper. While the human is moving, the BoneRenderer class continuously updates the bones for the skeletal pose view according to the human's joint positions. After all situations are created, the JSONParser class is called with all current scene data to serialize all information for the generated json as well as generate verbal embodied referral expressions according to what occurred in the scene. Please check the source code for further details regarding the way {\pa} simulator functions under the hood.

\subsection{Human Avatars and Skeletal Poses}
% shows a diagram of avatars and briefly describe
As one of the primary goals of our simulator {\pa} was to create a diverse dataset, we wanted our selection of humanoid characters to also promote diversity. Fig.~\ref{fig:avatars} shows all humans used for data generation, where multiple different races are used and the gender split is $50/50$.

\begin{figure}[!t]
    \centering
    \includegraphics[width=\columnwidth]{latex/images/human_display.png}
    \caption{Human avatars used to generated nonverbal interactions in {\pa} simulator. Eight different human avatars were used with four males/females as well as several different races.}
    \label{fig:avatars}
\end{figure}

  %\fbox{\includegraphics[clip, trim=1.5cm 12cm 1.5cm 7cm, width=\textwidth]{latex/images/stat_images/uml.drawio.pdf}}

Many other works have had success in interpreting embodied instructions through the use of skeletal poses. For example, \cite{chen2021yourefit} used a PAF heatmap to identify human gestural patterns. To accomplish this, we have added a gestural pattern camera to our simulator allowing for ground truth skeletal pose identification. This was accomplished by drawing lines between human bone joints using the Unity Vectrosity package \cite{unity_vectrosity}, as normal Unity line renderers have several limitations. Cameras from all 3 views (ego, exo, and top) were copied and modified to cull all layers except the layer the skeletal pose was drawn on, effectively creating a skeletal pose camera. This can be seen in Fig~\ref{fig:all_variation_samples}, where the human is made obvious to be pointing and gazing at an object towards the right.

%\subsection{Object Library}
% shows a diagram of object library and briefly describe

\subsection{Object Library for the {\dsxl} and {\dsl} datasets}
%add one para
While developing the {\pa} simulator, we decided to create an object library based on objects generally found in household environments. Thus, most objects in the {\dsxl} and {\dsl} datasets are commonly found in a kitchen, office, bathroom, or living room.  Additionally, a couple of unique objects were chosen to diversify further these datasets, such as a Decahedron or VR Headset. We display object libraries for both the {\dsl} dataset as well as the {\dsxl} dataset in Fig.~\ref{fig:object_lib_l} and Fig.~\ref{fig:object_lib_xl} respectively. Note that the object library for the {\dsxl} dataset (80 objects) is larger than the object library for the {\dsl} dataset (61 objects) due to the removal of duplicate object categories as well as certain small objects that were too difficult to identify by humans.

\color{blue}
All 80 objects in this library came from four purchased Unity Asset Store packages, that are linked below and covered under a Single Entity license. 
\begin{itemize}
    \item Furniture pack: \url{https://assetstore.unity.com/packages/3d/props/furniture/cabin-interior-household-items-furniture-pack-with-interactive-c-138278}
    
\item Fruits and vegetables pack: \url{https://assetstore.unity.com/packages/3d/props/food/pbr-fruits-and-vegetables-hdrp-158808}
\item Kitchen accessories pack: \url{https://assetstore.unity.com/packages/3d/props/interior/kitchen-accessories-200172}
\item Gluttony pack: \url{https://assetstore.unity.com/packages/3d/props/food/supermarket-gluttony-pack-12042}

\end{itemize}

\color{blue}

Additionally, we chose the object categories in this library carefully to ensure sufficient object diversity. Our object library contains objects we generally use in our daily life, such as kitchen and living room items, but also contains uncommon items, such as decahedrons  and VR devices. Moreover, as the home and kitchen items are diverse and graspable, the model trained on these data samples can be transferred for robotic learning to implement human-robot interactive systems.

\color{black}

\begin{figure}[!t]
    \centering
    \includegraphics[width=\textwidth]{latex/images/objects_L.png}
    \caption{The {\dsl} dataset Object Library, where a pool of $61$ objects are used. All objects found in {\dsl} are in {\dsxl}, with the extra $19$ objects in {\dsxl} being different versions of objects as well as some objects that were commonly too small to identify with a smaller resolution.}
    \label{fig:object_lib_xl}
\end{figure}

\begin{figure}[!t]
    \centering
    \includegraphics[width=\textwidth]{latex/images/objects_XL.png}
    \caption{The {\dsxl} dataset Object Library, where a pool of $80$ objects are used. Note that certain objects have multiple instances, such as pillow, cactus, and knife.}
    \label{fig:object_lib_l}
\end{figure}

%\subsection{Object Library}
% shows a diagram of object library and briefly describe

\subsection{Bounding Box Annotation}
As we can design the embodied referring expression comprehension task to identify a bounding box around the referred object \cite{chen2021yourefit}, creating tight bounding boxes was a priority. Extensive testing was done to ensure bounding boxes were as accurate as possible from all three views. A naive approach for extracting object bounding boxes in Unity is to use the corners of an object's mesh renderers. However, our testing found that these bounding boxes tended to be overestimates for bounding boxes, especially those from the ego view, as the ego camera was not aligned by global scene coordinate axes. Therefore the vertices of every object was checked relative to each camera to compute bounding boxes. This created much tighter and accurate bounding boxes.

This process was repeated for all three views to properly identify every object's location from every view. For both the exo and top view the cameras remain stationary, meaning this computation only needed to be performed once. However, the ego view camera constantly changes position and rotation according to where the human gazes, meaning these bounding boxes had to be computed dynamically. We decided to use Unity's physics synchronized update function for synchronizing bounding box calculations with video frames, since Unity's physics engine runs at a constant frame rate regardless of the frame rate of the engine. 
%we could synzhronize function calls with frames in the videos to label egocentric bounding boxes every frame. 

\subsection{Ambiguous Sample Generator}

Ambiguous samples, which differ from samples with contrasting instructions, are samples where the given modalities are not enough to completely identify the referred object. These were generated through supplying verbal utterances to the model in the \textit{No Human} scenario. For example, the scenario shown in Fig.~\ref{fig:all_variation_samples} along the \textit{No Human} row supplied with the verbal instruction ``the appl'' would be deemed as ambiguous as it is impossible to determine which apple is``the apple'' without knowing more information. However, the verbal instruction ``The red apple to the left of the black kettle'' would be deemed non-ambiguous as there is only one apple next to the cutting board.

\subsection{Additional Pointing Gesture Information}
Our hybrid pointing gesture approach allows us to generate novel motion it has no reference to, since it is unconstrained by a motion-capture library. It also ensures that generated motion obeys observed patterns in motion-capture data, like acceleration, gesture timing, and arc-like arm paths. Our model is based on the five-phase gesture model described in Kendon et. al's work \cite{Kendon1997gesture}, with gesture phases including rest, preparation, stroke, hold, and retraction phases. Finally, unlike many classical physical simulation algorithms, our simulator does not rely on overtly-complex mathematical modeling of musculo-skeletal forces, which both significantly would increase computational time, as well as diminish our control over the resulting motion, which often results in ``physically valid but unrealistic solutio'' \cite{Liu2005TowardsAG}. 

% Rather, the equation below was used to convert a Catmull Rom curve to a Bezier curve.

% \begin{equation}
%      \begin{bmatrix}
%           P'_0
%           \\P'_1
%           \\P'_2
%          \\ P'_3
%      \end{bmatrix}\caption{CatmullRom}
%      \xrightarrow{}
%      \begin{bmatrix}
%      P_1
%      \\P_1 + {P_2 - P_0}\over{6}
%      \\P_2 - {P_3 - P_1}\over{6}
%      \\P_2
%      \end{bmatrix}
%      \caption{Bezier}
% \end{equation}

\begin{figure}
\small
    \centering
    \begin{tabular}{c}
        \includegraphics[width=\columnwidth]{latex/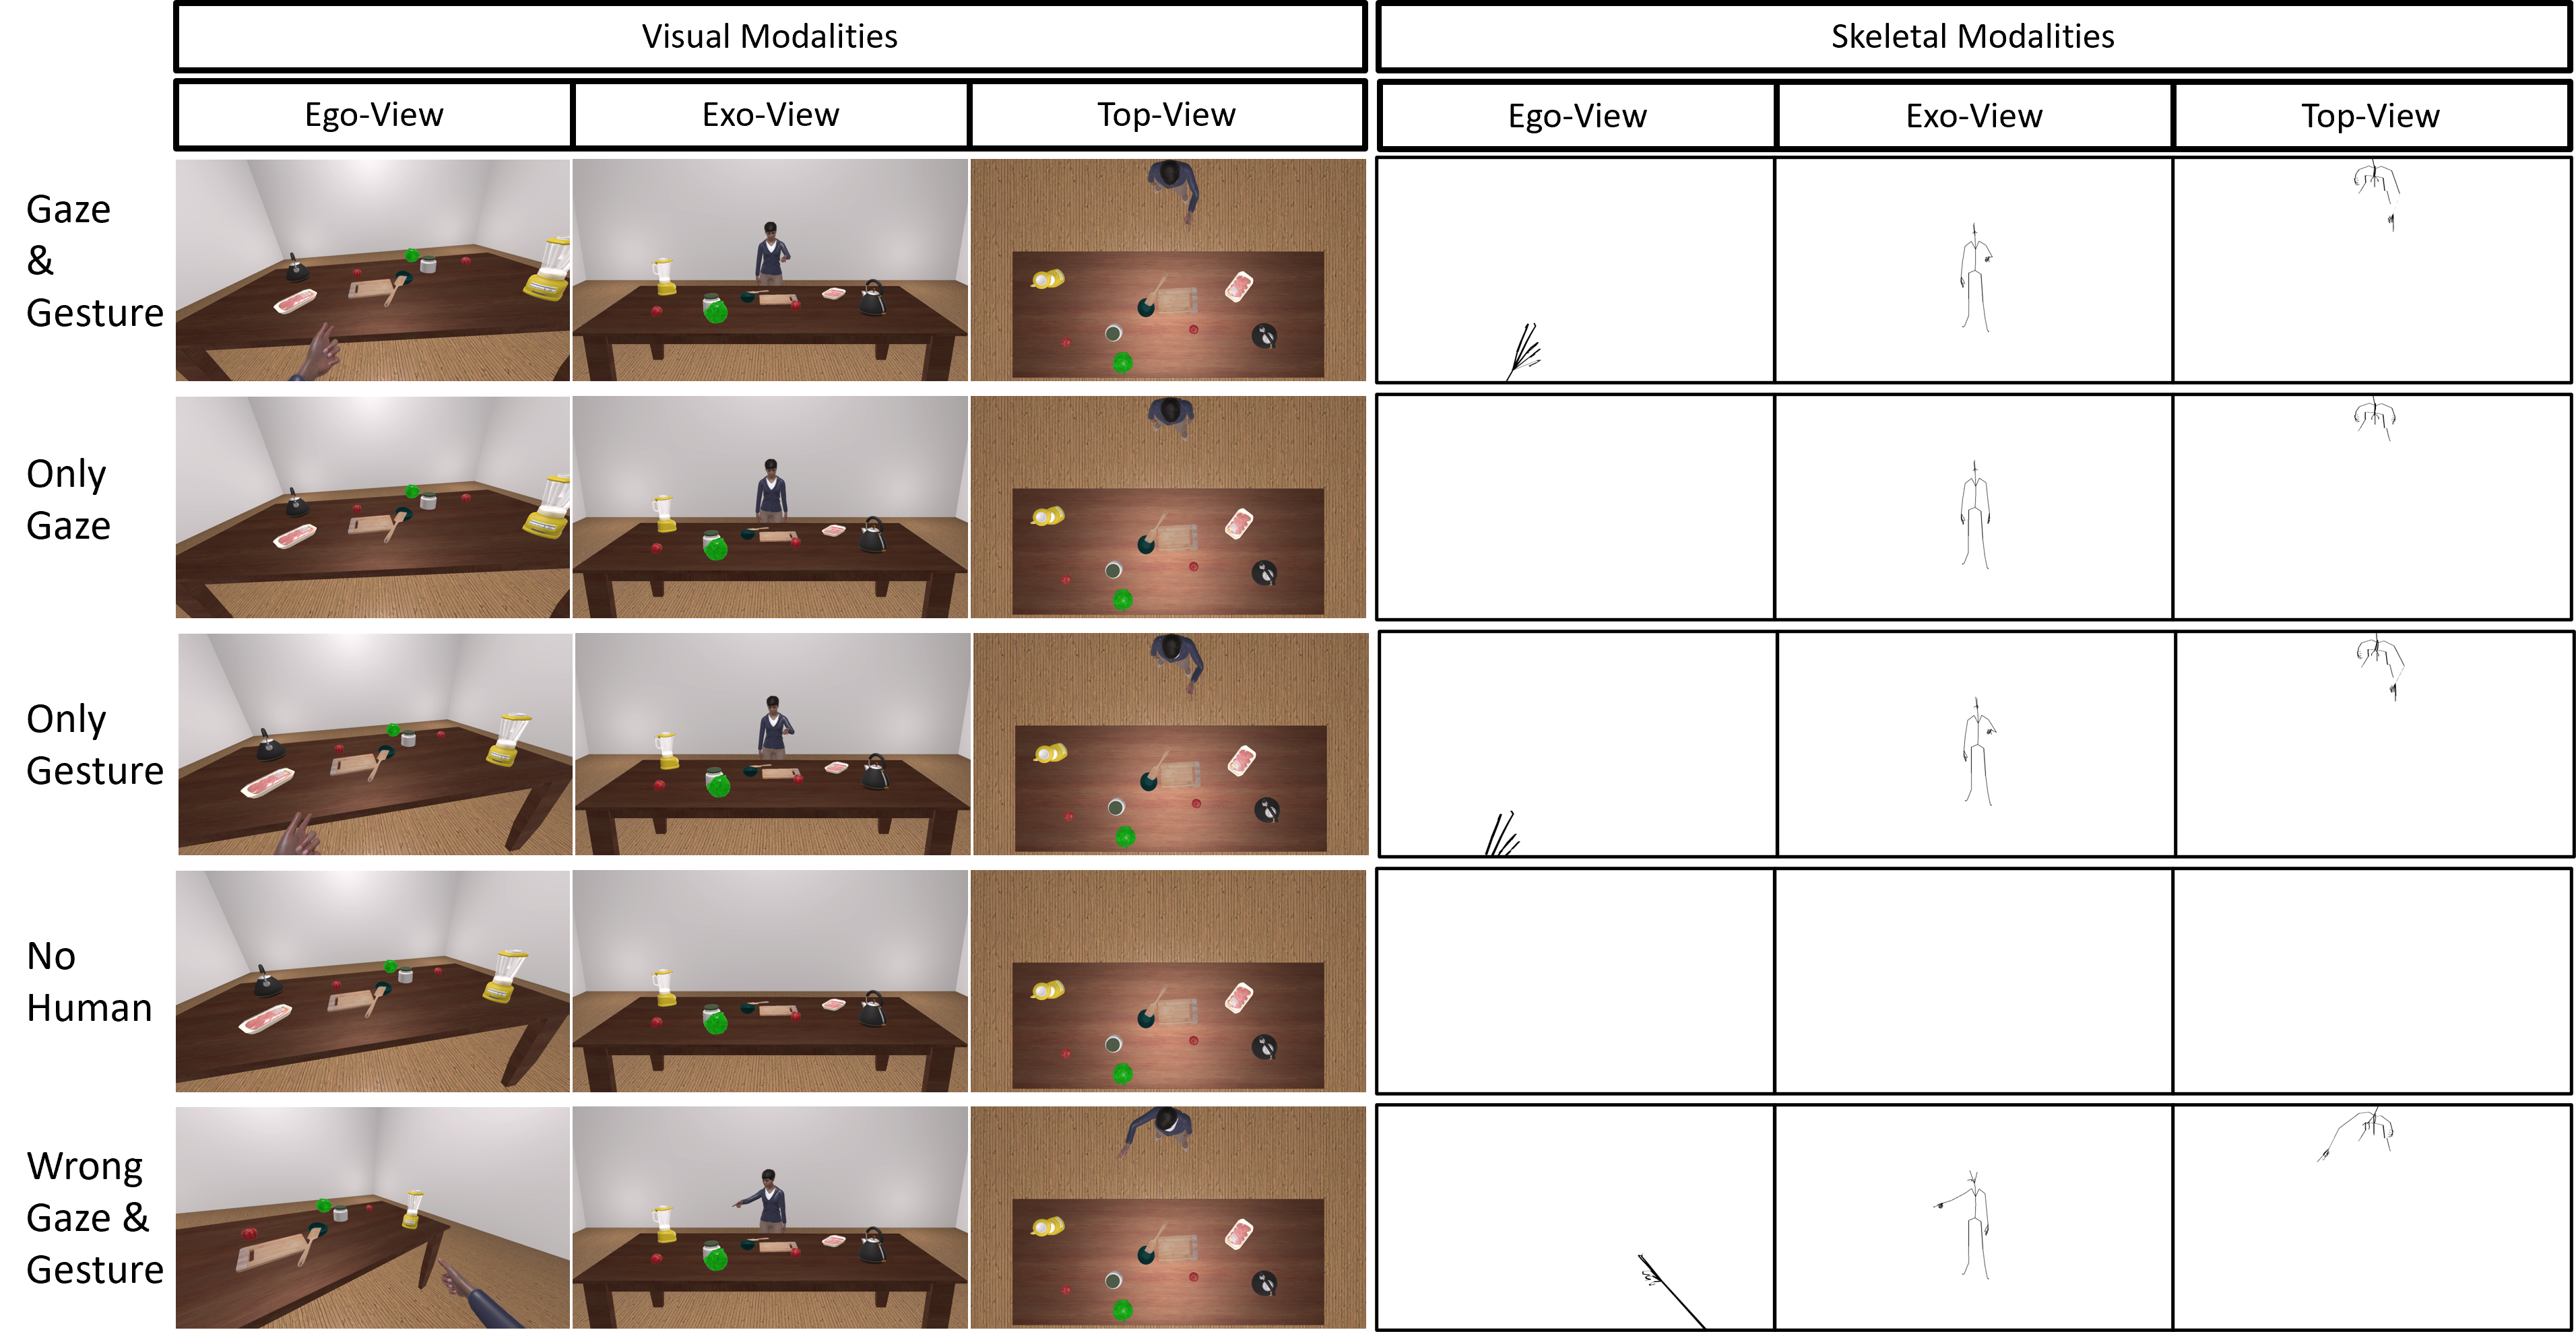}  \\
         Verbal utterance: The red apple to the left of the black kettle
    \end{tabular}
    \caption{Generated data using our simulator {\pa} by varying non-verbal modalities (gaze and pointing gesture). Note that for the case of No Human there are no skeletal poses as there is no human in the scene.}
    \label{fig:all_variation_samples}
\end{figure}

\subsection{Scalable Data Generation}
We wanted the {\pa} simulator to effectively use a resource-intensive cluster computing system to generate data at scale. Additionally, Unity supports multithreaded rendering. Thus, supporting parallel data generation within our simulator would allow users to configure the speeds by which they generate data based on their computing system. Allowing for configurable parallelization also allows for scalable data generation. To accomplish this, parallel data generation within our simulator is done by spawning another data generation scene with all necessary objects while other data generation scenes are running.

\section{Dataset Generation Procedure}
Data generation of a given data sample begins through the creation of a scene's environment, with the floor, table, human, and walls being dynamically loaded. Proceeding this, all objects are loaded in based on the methods described in the paper (Section 3.1). Next, data generation for the eight different scenarios \footnote{There are four synced scenarios where a verbal utterance and non-verbal gesture refer to the same object: Using gaze, pointing gesture, and verbal utterance; Using gaze and verbal utterance, Using pointing gesture and verbal utterance; Using verbal utterance and no human avatar. There are four more contrastive scenarios for the four described synced scenarios, where the verbal utterance and non-verbal gesture refer to different objects (note that for no human avatar as there is no non-verbal gesture an object not within the scene is referenced.} starts generating a human gaze or gesture (Section 3.2 in the paper). Moreover, we generate contrastive samples based on the procedure described in the paper (Section 3.4). While data is generating videos are recorded (if selected to in the {\ds} settings), canonical frames are saved, and bounding boxes are computed and stored. Once all situations have been completed, all labels are passed into a JSON parser, responsible for creating the string to serialize into a JSON. During this process the verbal utterance templates are used to generate utterances describing the referred objects (Section 3.2 in the paper). This process is done in parallel according to the number of times designated by the user in the {\ds} settings, discussed more in Section~\ref{section:data_gen_interface}. The entire data generation process is visualized in algorithm~\ref{algo:generate_data}.

\begin{algorithm}[!t]
\small
\KwIn{$T$: Total sample to generate; $S$: Number of parallel scenes designated in data generation settings}
\KwOut{$D$: Generated data sample}

$D \gets \emptyset $ \hfill\Comment{Generated dataset to empty}
\\
\For{$i \gets 1$ to $T$}{
    LoadAssets() \hfill\Comment{Load different assest, including objects, virtual avatars, etc.)} 
    \\
    GenerateObjects() \hfill\Comment{Randomly spawn objects at different locations}
    \\
    PrepareDifferentCamerasAndViews() \hfill\Comment{Initialize cameras to capture nonverbal interactions.}
    \\
    \For{$s \in S$}{
        PerformGazeOrGesture() \hfill\Comment{Render gaze and pointing gestures based on the referred object location.}
        \\
        CreateContrastiveSituation() \hfill\Comment{Generated contrastive data samples.}
        \\
        AnnotateImagesAndVideos()
    }
    $D \gets D \cup $ ParserData() \hfill\Comment{Parse data to json file to record data annotations.}
    \\
}
\textbf{return} Generated dataset, $D$
\caption{Data generation procedure in {\pa} simulator}
\label{algo:generate_data}

\end{algorithm}

% \begin{verbatim}
% while(total_samples_generated < total_samples_to_generate):
%     for i in range(# of parallel scenes):
%         LoadAssets()
%         GenerateObjects()
%         PrepareDifferentCamerasAndViews()
%         for j in range(# of situations):
%             GenerateData()
%         ParseData()
        
% def GenerateData():
%     PerformGazeOrGesture()
%     CreateContrastiveSituation()
%     AnnotateImagesAndVideos()
% \end{verbatim}
