# Supplementary material for: Embodied Referring Expression Comprehension in Human-Robot Interaction
Source: arXiv:2512.06558 source file (2025-12-06)
Supplement: Supplementary file 7 [file simulator_tool.tex]

\begin{table}[!h]
    \small
    \centering
    \begin{tabular}{p{0.17\linewidth}|p{0.75\linewidth}}
        \toprule
        Parameter &  \makecell{Explanation of Parameter} \\ \hline
        Object Pool & List of different objects to load into simulator. Does not use objects dragged into this field (loads all objects in Resources/objects folder) unless designated to by user in the \textit{Dynamically Load Object} parameter.\\ \hline
        Humans & List of different humans to choose at random.\\ \hline
        Tables & List of different tables to choose at random.\\ \hline
        Floor Materials & Different floor materials to choose at random.\\ \hline
        Parallel Scenes & Number of scenes generating data concurrently.\\ \hline
        Total Scenes Generated & Number of scenes to generate total.\\ \hline
        Dynamically Load Objects & If toggled will dynamically load objects from those dragged into the \textit{Object Pool} parameter.\\ \hline
        Record & If toggled records video rather than just recording single canonical frames for each situation.\\ \hline
        Activate Skeletal Camera & If toggled will activate skeletal pose cameras.\\ \hline
        Draw Bounding Boxes & If toggled will draw bounding boxes onto canonical frames (as a diagnostic).\\ \hline
        Png or Jpg & If toggled will save images/videos as png's, else will save images/videos as jpg's.\\ \hline
        Use Different Directory & If toggled will use a different directory specified in the \textit{Directory} parameter.\\ \hline
        Directory & The absolute directory to generate data in, start with a / do not end with a /.\\ \hline
        Width & The width of images to generate, must match the width specified in the resolution of the game tab inside Unity.\\ \hline
        Height & The Height of images to generate, must match the Height specified in the resolution of the game tab inside Unity.\\ \hline
        Origin Top L Or Bottom L & If toggled will generate bounding box coordinates from the top left, otherwise it will generate coordinates from the bottom left.\\ \hline
        Use Preloaded Scene & If toggled will not dynamically generate objects and a humanoid but will create nonverbal signals from the preloaded scene, not used to generate data.\\

        \bottomrule
    \end{tabular}
    \caption{Data generation interface with configurable parameters and descriptions. }
    \label{tab:configuration_settings}
\end{table}

\section{Configurable Data Generation Interface} \label{section:data_gen_interface}
While designing the simulator we wanted users to be able to configure settings of datasets they generate according to a variety of different model tasks. Thus, we have created an interface for configuring different settings of {\pa} via the inspector tab in Unity. To allow for environmental configuration, {\pa} dynamically loads all passed in humans/objects/floors/tables, so users can directly configure these. Additionally, we made various image setting configurations possible, various modalities possible to record/not record, and added general usability features. All configurable settings as well as a description for each setting can be found in Table~\ref{tab:configuration_settings}. Additionally, we have prepared a video demonstrating how to configure parameters as well as use {\pa} to generate data:
\url{https://youtu.be/KnKcpG7c2fk}.

% add table for all configuration settings
% how researchers can use our simulator tool to generate data
% we can record a short 1-2 min video and link here
