# Supplementary material for: Embodied Referring Expression Comprehension in Human-Robot Interaction
Source: arXiv:2512.06558 source file (2025-12-06)
Supplement: Supplementary file 8 [file appendix-a.tex]

\begin{figure*}[!h]
\centering
\includegraphics[scale=0.35]{images/data-anotation-system.png}
\caption{Data annotation tool}
\label{fig:data-anotation}
\end{figure*}

\newcommand{\FTdir}{}
\def\FTdir(#1,#2,#3){%
  \FTfile(#1,{{\color{black!40!white}\faFolderOpen}\hspace{0.2em}#3})
  (tmp.west)++(0.8em,-0.4em)node(#2){}
  (tmp.west)++(1.5em,0)
  ++(0,-1.3em) 
}

\newcommand{\FTfile}{}
\def\FTfile(#1,#2){%
  node(tmp){}
  (#1|-tmp)++(0.6em,0)
  node(tmp)[anchor=west,black]{\tt #2}
  (#1)|-(tmp.west)
  ++(0,-1.2em) 
}

\newcommand{\FTroot}{}
\def\FTroot{tmp.west}
\begin{figure}
\centering

\begin{tikzpicture}%

  \draw[color=black!60!white]
  \FTdir(\FTroot,root,Dataset){       % root: parent = \FTroot
    \FTdir(root,sub_id, Subject\_ID){ 
        \FTdir(sub_id,sess_id, Session\_ID){ 
         \FTdir(sess_id,int_id, Interaction\_ID) {
          \FTfile(int_id, audio.mp3)
          \FTfile(int_id, transcription.txt)
          \FTdir(int_id,vid,Videos){
            \FTdir(vid,rgb, RGB){
                \FTfile(rgb, exo.mp4)
                \FTfile(rgb, ego.mp4)
            }
            \FTdir(vid,depth, Depth){
                \FTfile(depth, exo.mp4)
            
            }
             \FTdir(vid,infrared, IR){
                \FTfile(infrared, exo.mp4)
            
            }
          
          }
            \FTdir(int_id,fid,Frames){
            \FTdir(fid,rgb, RGB){
                \FTfile(rgb, exo.jpg)
                \FTfile(rgb, ego.jpg)
            }
            \FTdir(fid,depth, Depth){
                \FTfile(depth, exo.jpg)
            
            }
             \FTdir(fid,infrared, IR){
                \FTfile(infrared, exo.jpg)
            
            }
          
          }
          \FTfile(int_id, acceleration.json)
          \FTfile(int_id, gyro.json)
          \FTfile(int_id, skeleton.json)
        
         }
    }
     
    }
  };
  \end{tikzpicture}
  \caption{Dataset folder structure}
  \end{figure}
